# Supplementary material for: Ultra high temperature superfluidity in ultracold atomic Fermi gases with mixed dimensionality
Source: arXiv:1807.05049 ancillary file (2018-09-08)
Supplement: Supplementary file 1 [file SI.pdf]

**Supplementary Information**

# Ultra high temperature superfluidity in ultracold atomic Fermi gases using mixed dimensionality


Leifeng Zhang,[1,2] Jibiao Wang,[3] Yi Yu,[4,1] and Qijin Chen[1,2,*]

[1] *Department of Physics and Zhejiang Institute of Modern Physics, Zhejiang University, Hangzhou, Zhejiang 310027, China*

[2] *Synergetic Innovation Center of Quantum Information and Quantum Physics, Hefei, Anhui 230026, China*

[3] *Laboratory of Quantum Engineering and Quantum Metrology, School of Physics and Astronomy, Sun Yat-Sen University (Zhuhai Campus), Zhuhai, Guangdong 519082, China*

[4] *Center for Measurements and Analyses, Zhejiang University of Technology, Hangzhou, Zhejiang 310014, China*



(Dated: September 8, 2018)



Here we present supplementary materials to the main text.


## I. RELATIONSHIP BETWEEN $1/k_F a$ AND $1/k_F a_{eff}$

In this section, we show an example plot of $a/a_{eff}$, which is the ratio between $1/k_F a_{eff}$ and $1/k_F a$, as a function of $k_F d$ for $t/E_F = 0.1$. The curve is presented in Fig. S1. For small $d$ (or small $td^2$ in general), the ratio approaches the value of 5/6.

## II. FERMI SURFACE MISMATCH IN MIXED DIMENSIONS

Mixed dimensionality necessarily causes Fermi surface mismatch between the two pairing components. For illustration purpose, shown in Fig. S2 is an example for $t = 0.01E_F$ and $k_F d = 8$ for the lattice component in the noninteracting limit, as compared with its 3D counterpart. The atoms form a disc (or cylinder) in the momentum space for these parameters. More cases can be found in Fig. 1 of Ref. [1]. Here the thickness of the disc is given by $2\pi/d$, and the dispersion on the out edge of the disc is controlled by $t$. For smaller $t/E_F = 0.0025$, the dispersion will be invisible in the plot.

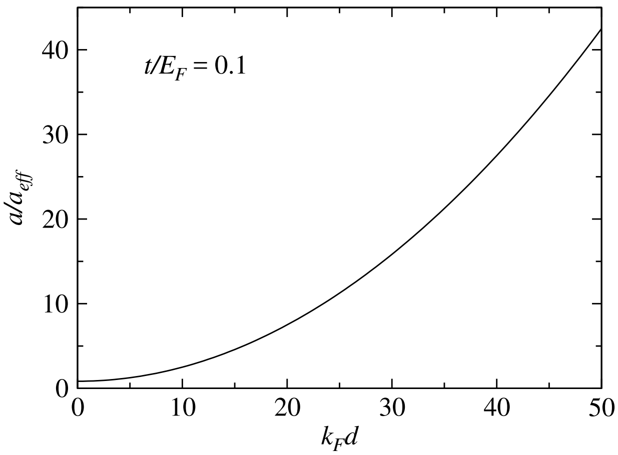


Figure S1. The ratio $a/a_{eff}$ as a function of $k_F d$ for $t/E_F = 0.1$.

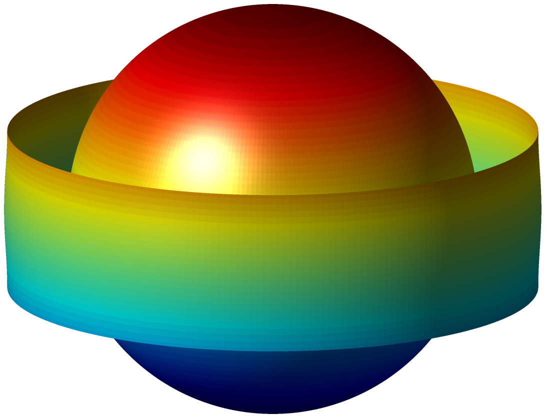

Figure S2. Elevated Fermi level for the lattice component with $t = 0.01E_F$ and $k_F d = 8$ in the noninteracting limit, as compared with its 3D counterpart (represented by the sphere). The lattice component occupies a quasi-2D Fermi disc in momentum space.

## III. BEHAVIOR OF THE EXCITATION GAP, EFFECTIVE PAIRING STRENGTH, AND CHEMICAL POTENTIAL AT THE MAXIMAL $T_c$ POINTS

In this section, we present the behavior of the excitation gap $\Delta(T_c)$, effective pairing strength $1/k_F a_{eff}$, and chemical potential $\mu_\sigma(T_c)$ of the 3D component at the maximal $T_c$ points for $2mtd^2 = 0.16$. The result is shown in Fig. S3. With increasing $d$, both the effective interaction strength $1/k_F a_{eff}$ and the corresponding gap $\Delta$ grow roughly linearly when $k_F d > 5$. At the same time, the chemical potentials $\mu_\uparrow$ and $\mu_\downarrow$ for the lattice and 3D components increases and decreases linearly, respectively. The increasing $\mu_\uparrow$ reflects the fact that a large $d$ pushes up the Fermi level of the lattice component. The decreasing $\mu_\downarrow$ reflects that the pairing grows stronger and enters the BEC regime. This is consistent with the increasing excitation gap $\Delta$ and increasing $1/k_F a_{eff}$.

## IV. MOMENTUM DISTRIBUTIONS FOR $t/E_F = 0.01$ AND $k_F d = 4$ BUT DIFFERENT PAIRING STRENGTHS

Shown in Fig. S4 is the momentum distribution of the 3D component, $n_\downarrow(k_\parallel, k_z = 0)$, in the $k_z = 0$ plane, for the


* Corresponding author: qchen@uchicago.edu

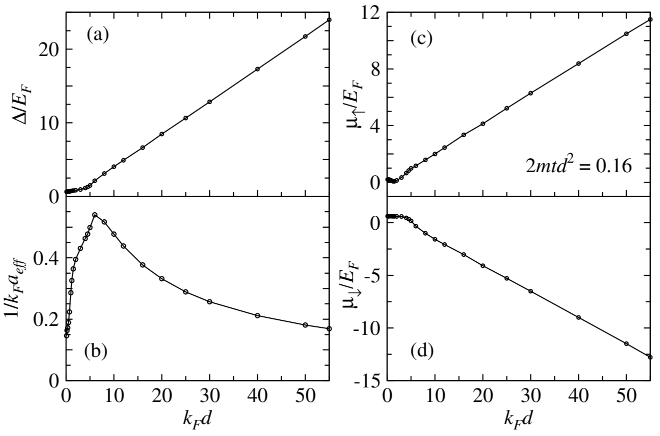


Figure S3. (a) Excitation gap $\Delta$, (b) $1/k_F a_{eff}$, (c) $\mu_\uparrow$ of the lattice component and (d) $\mu_\downarrow$ of the 3D component at the maximum $T_c$ point as a function of $k_F d$ for $2mtd^2 = 0.16$.

case of $t/E_F = 0.01$ and $k_F d = 4$, with different pairing strengths characterized by $1/k_F a$. As $1/k_F a$ increases from 0, the system enters the BEC regime, and the excitation gap increases accordingly. Therefore, the momentum distribution becomes more spread out toward high momenta as in the BCS mean-field theory. It is hard to tell the effect of a large $d$ from this figure while the pairing strength is increasing as well.

## V. MOMENTUM DISTRIBUTIONS FOR $2mtd^2 = 0.16$ AT THE MAXIMUM $T_c$ POINTS

Now we present the momentum distributions of the 3D component both along the $\hat{k}_z$ axis and in the $k_z = 0$ plane, for $2mtd^2 = 0.16$. Shown in Fig. S5 is the momentum distribution along the $k_z$ axis at the maximum $T_c$ points. It indicates that with increasing $d$, not only the first Brillouin zone

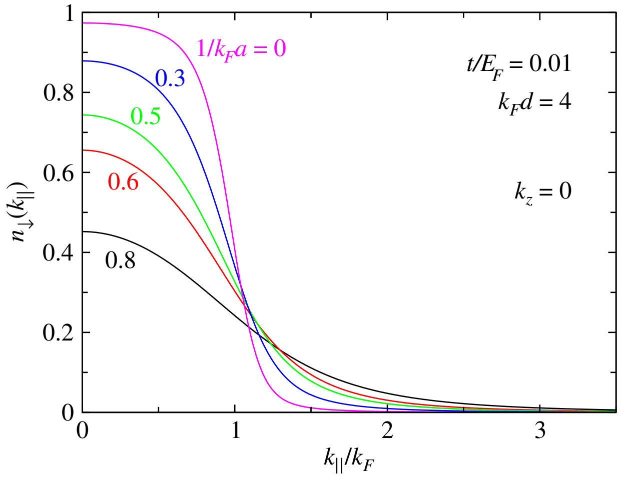


Figure S4. In-plane momentum distribution of the 3D component, $n_\downarrow(k_\parallel)$, in the $k_z = 0$ plane, for $t/E_F = 0.01$ and $k_F d = 4$, with different pairing strengths characterized by $1/k_F a$ (as labeled).

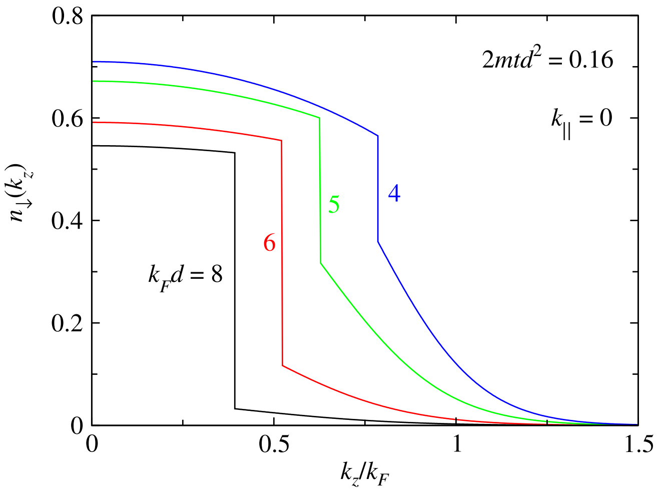


Figure S5. Momentum distribution of the 3D component along the $k_z$ axis at the maximum $T_c$ points for different $d$ and fixed $2mtd^2 = 0.16$. The step jumps occur at $k_z = \pi/d$.

boundary decreases but also that the spectral weight outside the zone decreases rapidly. In other words, the mismatch in the momentum distributions between the two pairing components at these maximum $T_c$ points is alleviated as $d$ increases. It is also interesting to note that to reach the maximum $T_c$, one does not necessarily need a perfect match in momentum distributions between the pairing fermions.

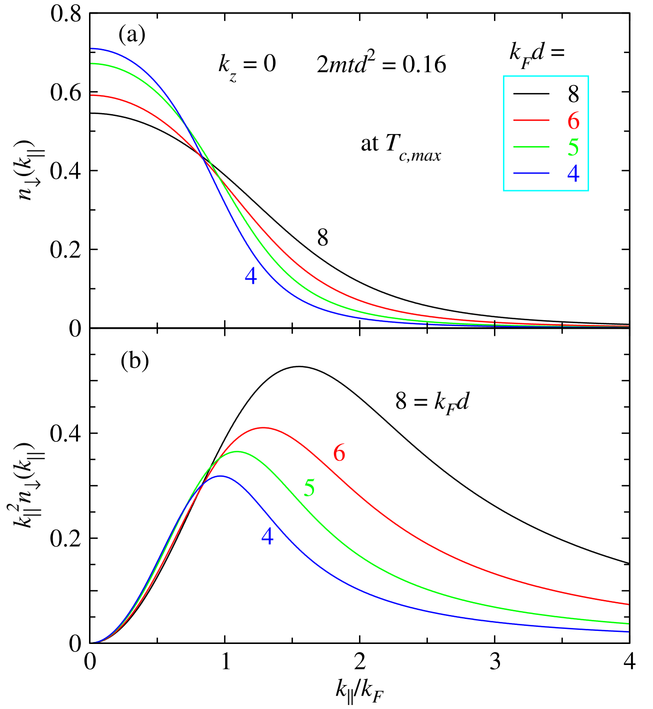


Figure S6. (a) Momentum distribution and (b) its second moment of the 3D component in the $k_z = 0$ plane at the maximum $T_c$ points for different values of $d$.

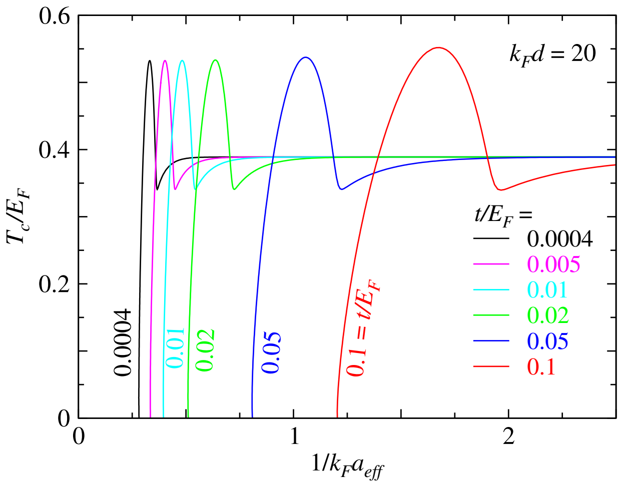


Figure S7. Effects of $t$ on the behavior of $T_c$ as a function of $1/k_Fa_{eff}$ for fixed $k_Fd = 20$ with different $t/E_F$ from 0.00004 up to 0.1.

Shown in Fig. S6(a) are the corresponding in-plane momentum distributions with $k_z = 0$. It is qualitatively not so much different from its pure dimensional counterpart; the curves are smooth, spanning from zero momentum all the way to infinity. In order to see the effect of a large $d$, we plot in Fig. S6(b) the second moment, $k_\parallel^2 n_\downarrow(k_\parallel, k_z = 0)$ as a function of $k_\parallel$ for this set of parameters. Now the peak of the second moment shifts progressively towards higher $k_\parallel$ values as $k_Fd$ increases. There is however also one complication that the effective interaction strength, $1/k_Fa_{eff}$, also changes simultaneously. From Fig. S3(b), $1/k_Fa_{eff}$ increases with $k_Fd$ for $k_Fd = 4, 5, 6$ and then starts to decrease for the $k_Fd = 8$ case. This complication may be removed by noting that the peak height also increases with increasing $d$, which necessarily leads to an increased occupation in the $k_x - k_y$ plane.

## VI. REPLOT OF FIG. 4 AS A FUNCTION OF $1/k_Fa_{eff}$

Here we represent Fig. 4 in the main paper as a function of $1/k_Fa_{eff}$, as shown in Fig. S7. Due to the relation between the bare parameter $1/k_Fa$ and the effective $1/k_Fa_{eff}$, these $T_c$ curves now exhibit different ordering horizontally.


[1] L. F. Zhang, Y. M. Che, J. B. Wang, and Q. J. Chen, "Exotic superfluidity and pairing phenomena in atomic Fermi gases in mixed dimensions," Sci. Rep. **7**, 12948 (2017).
